# Supplementary material for: Generalizable Deepfake Detection with Phase-Based Motion Analysis
Source: arXiv:2211.09363 source file (2022-11-17)
Supplement: Supplementary file 1 [file distortions_supp_cdfv2.tex]

\centering
%\begin{tabular}{ m{2cm} | m{0.5cm} | m{0.5cm} | m{0.5cm} | m{0.5cm} | m{0.5cm} | m{0.5cm} | m{0.5cm} | m{0.5cm} | m{0.5cm} | m{0.5cm} | m{0.5cm} | m{0.5cm} | m{0.5cm}}
\scalebox{0.9}{
\begin{tabular}{ m{2cm} | m{0.8cm} | m{0.8cm} | m{0.8cm} | m{0.8cm} | m{0.8cm} | m{0.9cm} | m{0.9cm} | m{0.8cm} | m{0.8cm} | m{0.8cm} | m{0.8cm} | m{0.9cm} | m{0.9cm}}

\Xhline{2\arrayrulewidth}
\tabledarkgray
\multicolumn{2}{c|}{}&\multicolumn{6}{c|}{\textbf{CDFv2}}&\multicolumn{6}{c}{\textbf{VFHQ}}\\
\hline
\multicolumn{2}{c|}{\textbf{Distortion}}&\multicolumn{2}{c|}{\textbf{CNN-GRU}}&\multicolumn{2}{c|}{\textbf{LipForensics}}&\multicolumn{2}{c|}{\textbf{PhaseForensics}}&\multicolumn{2}{c|}{\textbf{CNN-GRU}}&\multicolumn{2}{c|}{\textbf{LipForensics}}&\multicolumn{2}{c}{\textbf{PhaseForensics}}\\
\Xhline{2\arrayrulewidth}
type & level & auc & acc & auc & acc & auc & acc & auc & acc & auc & acc & auc & acc \\
\Xhline{2\arrayrulewidth}

\tablelightgray
&1&73.6&72.2&74.8&48.1&\textbf{89.5}&\textbf{80.7}&60.0&55.3&88.2&51.3&\textbf{94.6}&\textbf{74.3}\\
\tablelightgray
contrast&2&73.5&72.2&74.7&47.3&\textbf{90.0}&\textbf{79.2}&60.3&55.3&88.0&51.3&\textbf{94.5}&\textbf{76.3}\\
\tablelightgray
change&3&73.4&72.2&74.6&47.5&\textbf{89.4}&\textbf{75.9}&58.9&55.3&87.7&50.0&\textbf{94.7}&\textbf{75.7}\\
\tablelightgray
&4&73&72&74.2&47.9&\textbf{90.3}&\textbf{74.5}&59.5&55.3&87.4&50.0&\textbf{94.7}&\textbf{75.0}\\
\tablelightgray
&5&72.5&\textbf{71.2}&73.4&46.0&\textbf{89.1}&70.5&58.1&55.9&86.6&50.0&\textbf{95.3}&\textbf{78.3}\\

&1&70.5&65.1&72.8&46.9&\textbf{90.9}&\textbf{83.0}&46.2&54.6&90.3&52.0&\textbf{94.5}&\textbf{75.0}\\
color&2&69.4&62.4&72.2&47.3&\textbf{90.9}&\textbf{82.4}&42.0&52.6&90.4&52.0&\textbf{94.3}&\textbf{75.0}\\
saturation&3&67.8&61&71.7&49.0&\textbf{90.8}&\textbf{82.8}&37.1&49.3&90.5&52.0&\textbf{94.4}&\textbf{75.0}\\
&4&66&58.9&71.2&49.0&\textbf{90.6}&\textbf{82.2}&34.4&45.4&90.5&52.0&\textbf{94.4}&\textbf{75.0}\\
&5&63.9&58.3&70.1&47.9&\textbf{91.2}&\textbf{78.6}&33.7&44.1&90.5&51.3&\textbf{94.6}&\textbf{75.0}\\

\tablelightgray
&1&64.8&66.2&76.3&66.0&\textbf{91.3}&\textbf{66.8}&60.9&51.3&\textbf{96.5}&\textbf{80.3}&92.2&79.6\\
\tablelightgray
&2&62.7&66.8&74.6&66.4&\textbf{84.3}&\textbf{74.7}&59.5&51.3&\textbf{96.4}&\textbf{84.9}&72.9&64.5\\
\tablelightgray
pixelation&3&60.4&66.8&70.8&58.9&\textbf{78.7}&\textbf{69.5}&52.4&51.3&\textbf{94.2}&\textbf{80.9}&77.1&71.0\\
\tablelightgray
&4&60.4&66.2&67.9&\textbf{67.6}&\textbf{74.7}&65.8&49.8&50.0&\textbf{87.6}&\textbf{65.8}&66.3&\textbf{65.8}\\
\tablelightgray
&5&59.3&65.8&64.2&\textbf{68.2}&\textbf{67.9}&65.6&38.3&50.0&\textbf{83.8}&54.0&61.4&\textbf{61.8}\\

&1&70.5&67.2&\textbf{74.3}&49.0&72.6&\textbf{68.8}&56.6&56.6&\textbf{81.5}&\textbf{69.7}&81.3&67.1\\
&2&69.4&67.6&\textbf{72.2}&52.1&70.3&\textbf{69.0}&54.1&55.3&74.9&\textbf{70.4}&\textbf{78.9}&65.1\\
compression&3&66.4&64.1&\textbf{69.0}&55.0&64.6&\textbf{65.6}&51.5&54.0&71.4&61.8&\textbf{73.8}&\textbf{67.1}\\
&4&\textbf{64.1}&\textbf{65.3}&63.8&54.0&56.2&65.2&52.0&57.2&\textbf{66.9}&61.2&66.7&\textbf{61.8}\\
&5&\textbf{61.9}&\textbf{65.6}&61.1&50.0&50.1&65.4&52.4&49.3&62.2&56.6&\textbf{62.3}&\textbf{60.5}\\

\Xhline{2\arrayrulewidth}

\end{tabular}
}
