# Supplementary material for: Generalizable Deepfake Detection with Phase-Based Motion Analysis
Source: arXiv:2211.09363 source file (2022-11-17)
Supplement: Supplementary file 5 [file supp_adv_perturb.tex]

\centering
	\begin{tabular}[b]{ m{3cm} | m{2cm} |m{2cm} | m{2cm} |m{2cm}}
	
	\Xhline{2\arrayrulewidth}
	%\textbf{METHOD} &  FF++~\cite{Ros19} & FSh~\cite{LiL20A}  & DFor~\cite{Jia20} & DFDC~\cite{Dol20} & VFHQ~\cite{Fox21} &
	\tabledarkgray
	model & \multicolumn{2}{c|}{\textbf{CDFv2}} & \multicolumn{2}{c}{\textbf{FSh}}\\
	\tabledarkgray
	& \%auc $\uparrow$ & \%mape $\downarrow$ & \%auc $\uparrow$ & \%mape $\downarrow$ \\
	\hline
	CNN-GRU  & 43.4 & 37.8 & 49.7 & 38.5\\
	\tablelightgray
	LipForensics  & 49.5 & 39.9 & 62.7 & 35.4\\
	PhaseForensics  & \textbf{71.1} & 22.0 & \textbf{69.7} & \textbf{28.4}\\
\Xhline{2\arrayrulewidth}	
\end{tabular}
